# Supplementary material for: Safe Exploration for Efficient Policy Evaluation and Comparison
Source: arXiv:2202.13234 source file (2022-06-18)
Supplement: Supplementary file 1 [file 9_Appendix_other_settings.tex]

% $\vPhi_0$ is the design matrix in $\mD_0$ and 


% \begin{equation}
%     \begin{split}
% \argmin_{\vPhi} \;
% &var(\widehat{V}_{b,T}(\pi_1) - \widehat{V}_{b,T}(\pi_0) )\\
% &= \bar{\vphi}^T_{\Delta \pi}
%     \sigma^2 (\vPhi^T\vPhi + \vPhi_0^{T}\vPhi_0)^{-1} (\vPhi^T\vPhi) (\vPhi^T\vPhi + \vPhi_0^{T}\vPhi_0)^{-1}
%     \bar{\vphi}_{\Delta \pi_1}. 
%     \end{split}
% \end{equation}


% via the "FW G-optimal allocation" algorithm
% No matter whether $\mA$ is a fixed finite set of arms or $\mA=\mR^d$, the problem can be solved as in  . 

% We can then solve 
% % impose the constraint 
% \begin{equation}
%     \begin{split}
% &\argmin_{\vPhi} \;
% \bar{\vphi}^T_{\pi_1}
%     \sigma^2 (\vPhi^T\vPhi + \vPhi_0^{T}\vPhi_0)^{-1} (\vPhi^T\vPhi) (\vPhi^T\vPhi + \vPhi_0^{T}\vPhi_0)^{-1}
%     \bar{\vphi}_{\pi_1}\\
% &s.t. \; \min_{\vthe \in \mathcal{C}_\delta} \vone^T\vPhi \vthe \ge (1-\epsilon) T \times V(\pi_0).
%     \end{split}
% \end{equation}
% It remains to be derived how to solve this problem. 
% If not feasible, one heuristic approach is similar with the conservative bandit literature to solve from $t = 1$ to $T$ (go with the production policy when we will violate, and otherwise choose the one that minimize the variance). 
% % , by gradually decreasing $T$ until the solution of the unconstrained problem can satisfy the safety constraint (considering that. the remaining budgets will be used on the production policy). 


%%%%%%%%%%%%%%%%%%%%%%%%%%%% Offline dataset not useful here? %%%%%%%%%%%%%%%%%%%%%%%%%%%%
% With $\widehat{V}(\pi) = (T+N)^{-1} \{\sum_{t=1}^T \frac{\pi(A_t)}{b(A_t)}R_t + 
% \sum_{i=1}^N \frac{\pi(a_i)}{b_0(a_i)} R'_i
% \}$, 
% we have 
% \begin{equation}
%     \begin{split}
%         T \times var(\widehat{V}_{b,T}(\pi_1) - \widehat{V}_{b,T}(\pi_0) \mid \{a_i\}_{i=1}^N)
%         % &= var(\sum_t \frac{\pi_{\Delta}(A_t)}{b(A_t)}R_t )\\
%         &= var(\frac{\pi_{\Delta}(A_t)}{b(A_t)}R_t )\\
%         &= 
%         \Mean_{A_t \sim b}[var(\frac{\pi_{\Delta}(A_t)}{b(A_t)}R_t \mid A_t)]
%         + var_{A_t \sim b}[\Mean(\frac{\pi_{\Delta}(A_t)}{b(A_t)}R_t \mid A_t)]\\
%         &= 
%         \Mean_{A_t \sim b}[\frac{\pi^2_{\Delta}(A_t)}{b^2(A_t)}var(R_t \mid A_t)]
%         + var_{A_t \sim b}[\frac{\pi_{\Delta}(A_t)}{b(A_t)}r(A_t)]\\
%         &= 
%         \sum_a \big[\frac{\pi^2_{\Delta}(a)}{b(a)}var(R_t \midA_t = a) \big]
%         + var_{A_t \sim b}[\frac{\pi_{\Delta}(A_t)}{b(A_t)}r(A_t)]\\
%         % &= \sum_t 
%         % \Big\{
%         % var[\frac{\pi_{\Delta}(A_t)}{b(A_t)}r(A_t)]
%         % \Big\} + const\\
%     \end{split}
% \end{equation}



% \begin{equation}
%     \begin{split}
%         &\argmin_{b' \ge \vzero} \sum_a \frac{\pi^2_{\Delta}(a)}{(1-\epsilon) \pi_0(a) + b'(a)} \\
%         % var_{A_t \sim b}[\frac{\pi_{\Delta}(A_t)}{b(A_t)}r(A_t)]\\
%         &s.t. \;\; \sum_a b' = \epsilon 
%         % V(b) \ge (1-\epsilon) V(\pi_0). 
%     \end{split}
% \end{equation}

% \begin{equation}
%     \begin{split}
%         &\argmin_b \sum_a \pi^2_{\Delta}(a) b^{-1}(a) \\
%         % var_{A_t \sim b}[\frac{\pi_{\Delta}(A_t)}{b(A_t)}r(A_t)]\\
%         &s.t. \;\; b^{-1} \le (1-\epsilon) \pi^{-1}_0\\
%         & \;\;\;\;\;\;\; b^{-1} \ge \vone_K
%         % V(b) \ge (1-\epsilon) V(\pi_0). 
%     \end{split}
% \end{equation}

% \section{Bayesian SafeOD}
% Our analysis so far is worst-case, i.e., we assume the designer will first choose $b$ and then the adversarial (the nature) will choose the instance. 
% Suppose we revert the roles, and consider that a distribution over $\vr$ is chosen at the first place, and then the designer will choose the strategy, then we are considering the Bayesian setup. 


Because we are targeting a non-adaptive exploration policy, 
the decision to go with the production policy is either a fixed proportion, or a more adaptive one. 
% Otherwise, we may consider the distributional G-optimal design in \cite{ruan2021linear}. 
% Why no information of $\vR$ here?



Differentiable policy $b(a\mid\vx)$ and optimize with SGD?
% Seems feasible to solve via simulation (Monte Carlo). 


% Not that correct. We have an existing dataset!




%%%%%%%%%%%%%%%%%%%%%%%%%%%%%%%%%%%%%%%%%%%%%%%%%%%%%%%%%%%%%%%%%%%%%%%%%%%%%%%%%%%%%%%%%%%%%%%%%%%%%%%%%%%%%%%%%%%%%%%%%%%%%%%%%%%%%%%%%%%%%%%%
% \textbf{Goal I (pure exploration for off-policy optimization, with fixed budget $T$). } 
% We would like to design a fixed policy $b$ to collect a new dataset $\mD = \{(\vx_t, A_t, R_t)\}_{t=1}^T$ where $A_t \sim b(\cdot\mid\vx_t)$, 
% so that after the $T$ interactions, 
% our new policy $\pi' = \mathcal{O}\Big(\mD \bigcup \mD\Big)$ will yield high value in expectation (or high-probability bound?), i.e., we aim to maximize $\Mean(V(\pi'))$ where the expectation is taken over $\mD$ and hence $\pi'$. 

% \textbf{Goal II (pure exploration for off-policy optimization, with fixed budget $T$ and safety constraint $\epsilon$). } 


% We would like to design a fixed policy $b$ to collect a new dataset $\mD = \{(\vx_t, A_t, R_t)\}_{t=1}^T$ where either $A_t \sim b(\cdot\mid\vx_t)$ or $A_t \sim \pi_0(\cdot\mid\vx_t)$, 
% so that after the $T$ interactions, 
% we satisfy the safety constraint that $\sum_t\Mean( R_t) \ge (1-\epsilon) \sum_t\Mean(R_t\mid\vx_t, \pi_0(\vx_t))$ and 
% our new policy $\pi' = \mathcal{O}\Big(\mD \bigcup \mD\Big)$ also yield high value in expectation (or high-probability bound?), i.e., we aim to maximize $\Mean(V(\pi'))$ where the expectation is taken over $\mD$ and hence $\pi'$. 

%%%%%%%%%%%%%%%%%%%%%%%%%%%%%%%%%%%%%%%%%%%%%%%%%%%%%%%%%%%%%%%%%%%%%%%%%%%%%%%%%%%%%%%%%%%%%%%%%%%%%%%%%%%%%%%%%%%%%%%%%%%%%%%%%%%%%%%%%%%%%%%%


% \begin{align*}
%     \argmin_{b} \; &\Mean_{\vx_t \sim p(\vx), A_t \sim b(a \mid \vx_t) }\Big(\frac{R_t  \pi_1(A_t \mid \vx_t)}{b(A_t \mid \vx_t)} \Big)^2\\
%     &= 
%     \Mean_{\vx_t \sim p(\vx)} \Big\{
%     \Mean_{A_t \sim b(a \mid \vx_t) } 
%     \frac{R^2_t  \pi^2_1(A_t \mid \vx_t)}{b^2(A_t \mid \vx_t)} 
%     \Big\}
%     \\
%     &= 
%     \Mean_{\vx_t \sim p(\vx)} \Big\{
%     \Mean_{A_t \sim \pi_1(a \mid \vx_t) } 
%     \frac{\Mean[R^2_t \mid \vx_t, A_t]  \pi_1(A_t \mid \vx_t)}{b(A_t \mid \vx_t)} 
%     \Big\}
%     \\
%     % s.t. \quad 
%     s.t. \; &\min_{\vthe \in \mathcal{C}_\delta} \quad \Mean_{\vPhi \sim b} \big(\vone^T \vPhi\vthe\big)  
%     \ge (1-\epsilon) \max_{\vthe \in \mathcal{C}_\delta}  \Mean_{\vPhi \sim \pi_0} \big(\vone^T \vPhi\vthe\big)  
%     % &XX1
% \end{align*}

%%%%%%%%%%%%%%%%%%%%%%%%%%%%%%%%%%%%%%%%%%%%%%%%%%%%%%%%%%%%%%%%%%%%%%%%%%%%%%%%%%%%%%%%%%%%%%%%%%%%%%%%%%%%%%%%%%%%%%%%%%%%%%%%%%%%%%%%%%%%%%%%
